# Supplementary material for: Hybrid antiferroelectric-ferroelectric domain walls in noncollinear antipolar oxides
Source: arXiv:2507.01622 source file (2025-07-02)
Supplement: Supplementary file 1 [file supplement_comp.pdf]

# Supplementary Information

## Hybrid antiferroelectric–ferroelectric domain walls in noncollinear antipolar oxides

Ivan N. Ushakov[1], Mats Topstad[2], Muhammad Z. Khalid[1], Niyorjyoti Sharma[3], Christoph Grams[4], Ursula Ludacka[1], Jiali He[1], Kasper A. Hunnestad[1,5], Mohsen Sadeqi-Moqadam[1], Julia Glaum[1], Sverre M. Selbach[1], Joachim Hemberger[4], Petra Becker[6], Ladislav Bohatý[6], Amit Kumar[3], Jorge Íñiguez-González[7,8], Antonius T. J. van Helvoort[2], and Dennis Meier[1]

[1]Department of Materials Science and Engineering, Norwegian University of Science and Technology (NTNU), Trondheim, Norway

[2]Department of Physics, Norwegian University of Science and Technology (NTNU), Trondheim, Norway

[3]Centre for Quantum Materials and Technologies (CQMT), Queen's University Belfast, Belfast, United Kingdom

[4]Institute of Physics II, University of Cologne, Cologne, Germany

[5]Department of Electronic Systems, Norwegian University of Science and Technology (NTNU), Trondheim, Norway

[6]Institute of Geology and Mineralogy, University of Cologne, Cologne, Germany

[7]Smart Materials Unit, Luxembourg Institute of Science and Technology (LIST), Esch/Alzette, Luxembourg

[8]Department of Physics and Materials Science, University of Luxembourg, Belvaux, Luxembourg

# Supplementary Note 1

### Electromechanical tensor calculations

For the calculations, we used density functional theory (DFT) within the PBEsol approximation [1] as implemented in VASP [2]. The atomic cores were treated using the projector augmented wave approximation, considering at least the following electrons explicitly in the calculations: 3p and 4s for K; 4p, 4d and 5s for Nb; 2s and 2p for B; and 2s and 2p for O. The electronic wave functions were described with a plane-wave basis cut off at 500 eV or higher. Reciprocal space integrals – for the high-temperature phase with a 20-atom unit cell – were computed using a grid of at least 3x3x6 k-points in the Brillouin zone (or similarly dense grids when other supercells were considered). Structural relaxations were stopped for residual forces and stresses smaller than $10^{-2}$ eV/Å and 1 kB, respectively. We note that two different groups (in Norway and Luxembourg) ran DFT simulations in this project, always using calculation conditions that are sufficiently converged, obtaining consistent results.

The piezoelectric and Born tensors were calculated within the framework of density functional perturbation theory (DFPT). $K_3[Nb_3O_6|(BO_3)_2]$ belongs to the 2mm point group and has three independent dielectric tensor components, five independent piezoelectric tensor components, and nine independent elastic stiffness components. The calculated tensor components used for FEM simulations are summarized in Tab. S1.

Table S1: Numerical values of the non-zero dielectric, piezoelectric, and elastic tensor components in the orthorombic phase of $K_3[Nb_3O_6|(BO_3)_2]$, calculated using DFT. The Voigt convention 4 = 23 = 32, 5 = 13 = 31, 6 = 12 21 is used.

| Dielectric tensor | | Piezoelectric tensor (pm/V) | | Elastic tensor (GPa) | |
|---|---|---|---|---|---|
| $\epsilon_{11}$ | 28.025 | $d_{11}$ | 1.52 | $C_{11}$ | 275.3 |
| $\epsilon_{22}$ | 27.685 | $d_{12}$ | -1.48 | $C_{12} = C_{21}$ | 107.1 |
| $\epsilon_{33}$ | 32.972 | $d_{13}$ | -0.011 | $C_{13} = C_{31}$ | 75.3 |
| | | $d_{26}$ | -3.195 | $C_{22}$ | 281.6 |
| | | $d_{35}$ | 0.84 | $C_{23} = C_{32}$ | 72.5 |
| | | | | $C_{33}$ | 157.7 |
| | | | | $C_{44}$ | 17.55 |
| | | | | $C_{55}$ | 17.65 |
| | | | | $C_{66}$ | 86.28 |

## Finite element modeling

The numerical modeling in Fig. 3(b) in the main text was conducted using a finite element solver integrated into COMSOL Multiphysics (Ver. 6.1). The piezoelectric sample was assumed to be a block with dimensions 500x250x200 nm with the same domain structure as in Fig. 3(a) and planar domain walls. The sample was characterized by assigning $P_a = 0.03$ $\mu$C/cm$^2$, and a complete set of piezoelectric, dielectric, and elastic tensors from Tab. S1. The tip was modeled as a cylinder with a contact radius of 5 nm (value based on the Hertz contact model with experimental parameters) and a height of 1 nm. Mesh refinement in proximity of the tip was conducted sequentially until mesh independence was achieved at approximately 11000 elements. For the elastic equation, the bottom face of the sample was assumed to be fixed. For the electrostatic equation, the lower face of the tip was assumed to have a biased potential of -5 V, whilst the bottom face of the sample was grounded. To simulate the PFM scan operation, a series of simulations were conducted along the path illustrated in Fig. 3(a) in the main text. With this quasi-static approach, the areal average of vertical displacement over the area of the tip's bottom face was calculated in different points of the path.

# Supplementary Note 2

### Tomographic AFM

We observed no substantial changes (like domain curving, merging, or separating) through the depth of 4 μm. Therefore, three out of the seven images (at 250 nm, 1 μm and 3 μm, Supplementary Fig. S7(a-c)) were chosen to construct Fig. 2(f) in the main text. Firstly, domain walls were isolated from each of the PFM images, then alpha shape triangulation was performed in MATLAB to form a 3D structure.

Additional information: Occasionally, AFM polishing succeeded the milling step to minimize the topographical crosstalk in the imaging stage. In this step, sequential reduction of deflection setpoint was done over a few scans to slowly lower the tip force on the surface and thus smoothening the milled area.

### Vector PFM

Vector PFM was performed by doing LPFM on the (001) sample face of $K_3[Nb_3O_6|(BO_3)_2]$ at different sample-cantilever angles ($\beta$ in Supplementary Fig. S2(a)). The signal strength within a domain is proportional to $\mathbf{P}\cdot\mathbf{v} = P\cos(\beta-\alpha)$, meaning that two domains, e.g., T′ and T″, would have the same contrast only if the condition $\cos(\beta-\alpha') = \cos(\beta-\alpha'')$ is met. We found three angles $\beta_1$, $\beta_2$, $\beta_3$ (Supplementary Fig. S2(b-d)), at which different domain pairs have the same contrast. The polarization angles $\alpha'$, $\alpha''$, $\alpha'''$ for the three domains then satisfy:

$$\begin{bmatrix}1 & 1 & 0\\ 0 & 1 & 1\\ 1 & 0 & 1\end{bmatrix}\begin{bmatrix}\alpha'\\ \alpha''\\ \alpha'''\end{bmatrix} = 2\begin{bmatrix}\beta_1 + 180^\circ n_1\\ \beta_2 + 180^\circ n_2\\ \beta_3 + 180^\circ n_3\end{bmatrix};\quad (n_1, n_2, n_3) \in \mathbb{Z}^3 \tag{1}$$

We find this equation to have two non-equivalent solutions, consistent with the two possible polarities of the PFM calibration (polarity of vector $\mathbf{v}$). We then find that the inequalities in Supplementary Fig. S2(b-d) satisfy the solution $\alpha' = -60^\circ$, $\alpha'' = 180^\circ$, $\alpha''' = 60^\circ$, which gives us the in-plane polarization directions.

### Vertical piezoresponse in bended domain walls

Vertical PFM was performed with the DART (Dual Amplitude Resonance Tracking) mode over a spot with two bended domain walls, shown in Supplementary Fig. S9(a). To enhance image quality, 28 images (7 scans) were averaged, as shown in Supplementary Fig. S9(b). At each scanning line, a cross section was extracted and its baseline was subtracted with

a node spacing of 10 pixels, and ± 30 pixels around the peak, as shown in Supplementary Fig. S9(c). The local domain wall intensity was then defined at the absolute maxima of the substracted peak, also defining the position of the domain walls. An example of a baseline substraction from a cross section in Supplementary Fig. S9(b) is shown in Fig. S9(c-d) in the main text, showing lower absolute intensity at a bended heah-to-head domain wall than on a straight tail-to-tail domain wall.

The domain wall angles at each scanning line were then found by smoothing domain wall profiles with a Savitzky–Golay filter and performing numerical differentiation. The intensity was finally plotted against the domain wall angle, as shown in Fig. 5(e-f) in the main text.

# Supplementary Figures

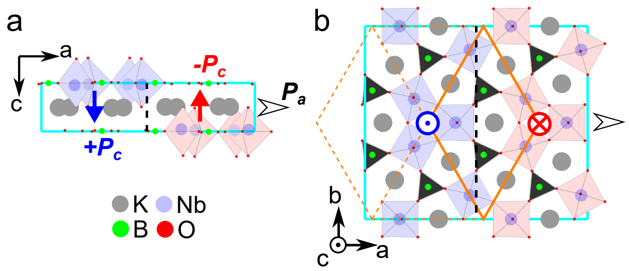


Figure S1: **Room-temperature unit cell of $K_3[Nb_3O_6|(BO_3)_2]$.** a) The canted antipolar arrangement in the *ac*-plane is presented. b) A perfect nearest-neighbor antipolar arrangement of the Nb-trimers in the ab-plane is forbidden by geometry. Antipolar order breaks the threefold symmetry of the high-temperture phase (orange cell), turning the material polar.

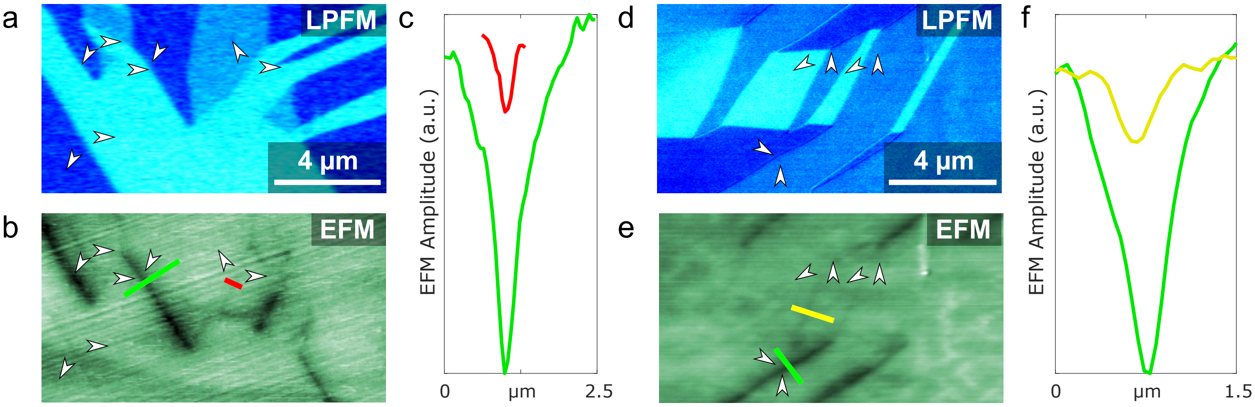


Figure S2: **Electrostatic response at tail-to-tail and head-to-tail domain walls.** a-b) LPFM and EFM of a (001) face region with both head-to-head and tail-to-tail domain walls. For visibility, the rows in b) have been aligned using a one-dimensional polynomial. c) EFM signal of the cross-sections in b), showing that the electrostatic signal measured at head-to-head walls is about 5 times stronger than at tail-to-tail walls. d-e) LPFM and EFM of a (001) face region where some head-to-tail domain walls are visible. f) Cross-sections from e).

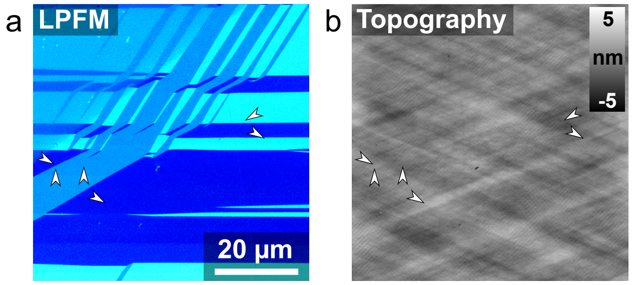


Figure S3: **Topography of polished samples.** a-b) LPFM and AFM, respectively, of the (001) sample face, showing that there are no signatures of domains and domain walls in the topography.

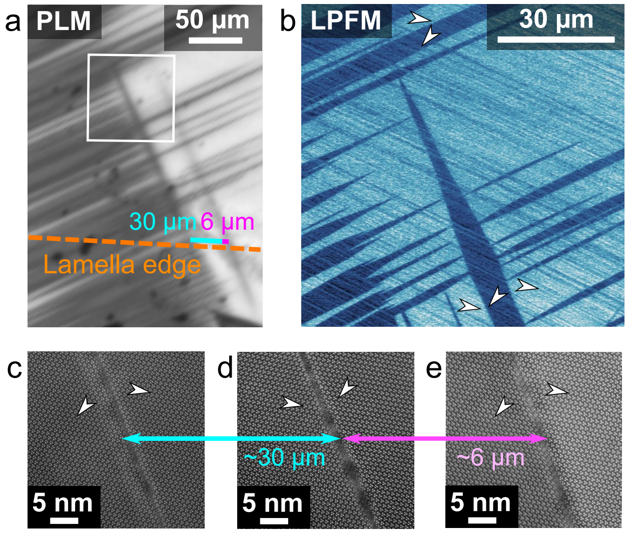


Figure S4: **Correlated PLM-PFM-STEM studies and determination of domain wall types in TEM.** a) PLM image of a (001) sample face before a wedge lamella was prepared. The distance to one needle-like domain and its thickness is shown. b) LPFM of the white square in a), used to determine the polarization directions and the three domain wall types. c-e) Domain walls were observed with the same spacing as shown in a), allowing to determine the type of these domain walls. Note that no head-to-tail walls were observed in TEM, although expected on the lamella edge. Furthermore, the TEM data confirms that the effective shear piezocoefficient is positive with respect to the antipolar canting $P_a$.

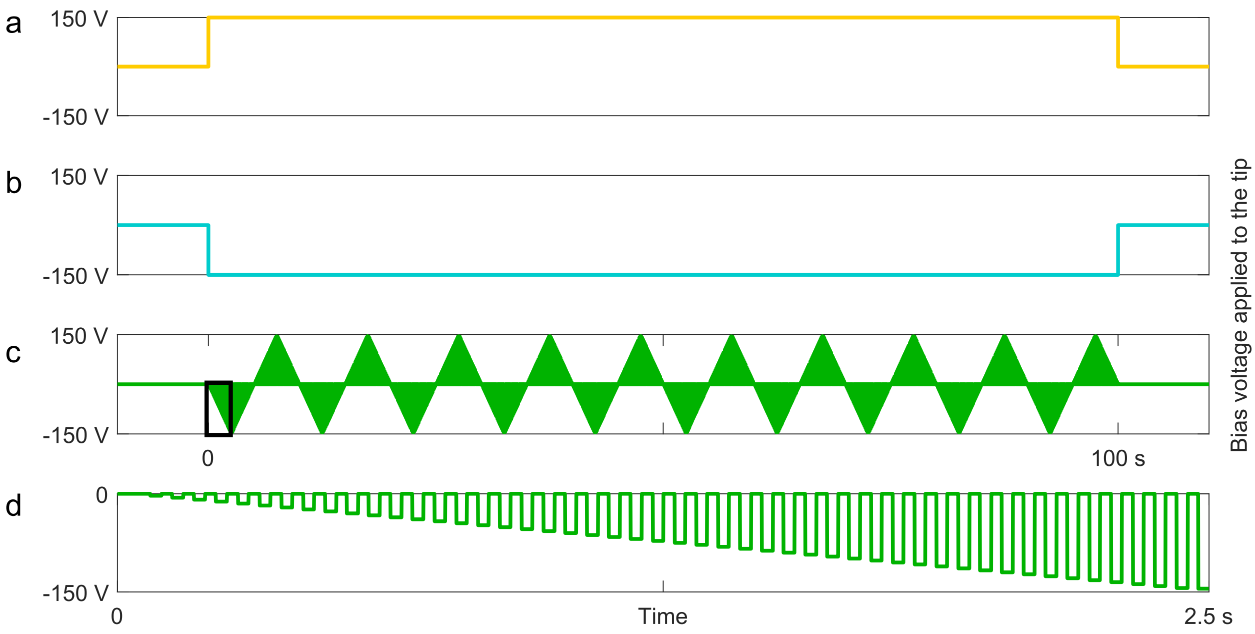


Figure S5: **Bias profiles used for domain wall bending.** a) Positive DC bias. b) negative DC bias. c) AC bias. d) Zoom-in to the black square in c), showing that the AC bias is made up of linearly decreasing/increasing step pulses, having 200 steps per period (=10 s) and 10 periods in total.

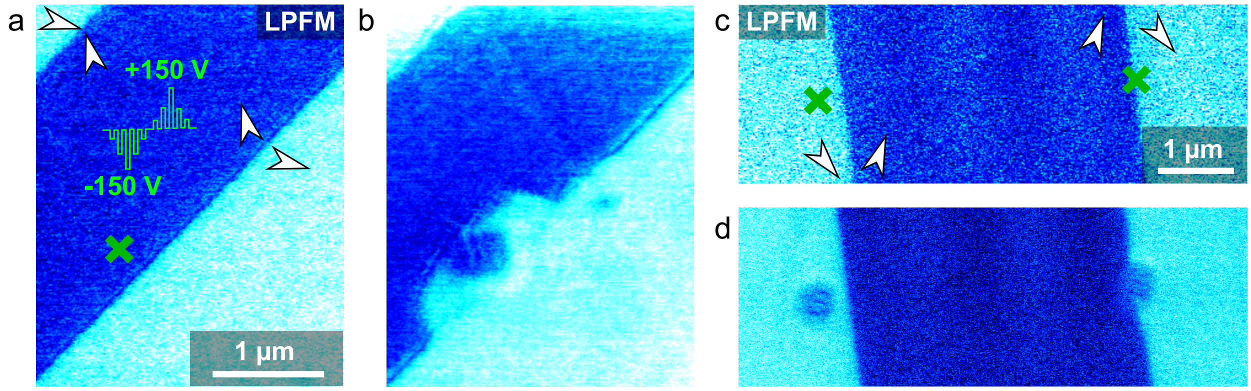


Figure S6: **Domain wall bending.** a-b) Tail-to-tail domain wall moving towards its nearest neighbor, even when bias is applied between the walls. the same effect is observed for head-to-head domain walls (not shown). c-d) The mobility of head-to-tail domain walls is negligible.

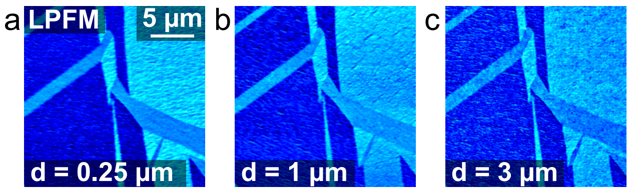


Figure S7: **Cross-sections in tomographic AFM.** a-c) Lateral PFM plotted as $A\cos\phi$ at the three milling depths used for 3D reconstruction in Fig. 2(f) in the main text.

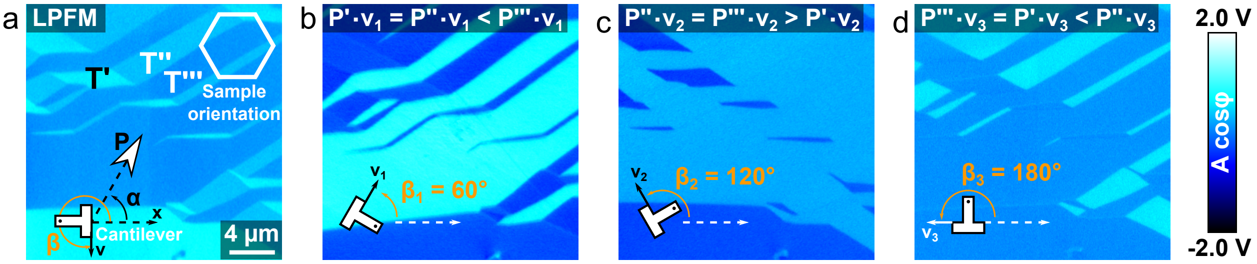


Figure S8: **Vector PFM procedure.** The opposite calibration convention from Ref. [3] was used, making the domain signal positively proportional to its in-plane polarization component **P** projected on the vector **v** in a). With three domains in total, we found three sample-cantilever orientations in b-d), where different domain pairs give the same contrast, giving the denoted signal strength equations and inequalities.

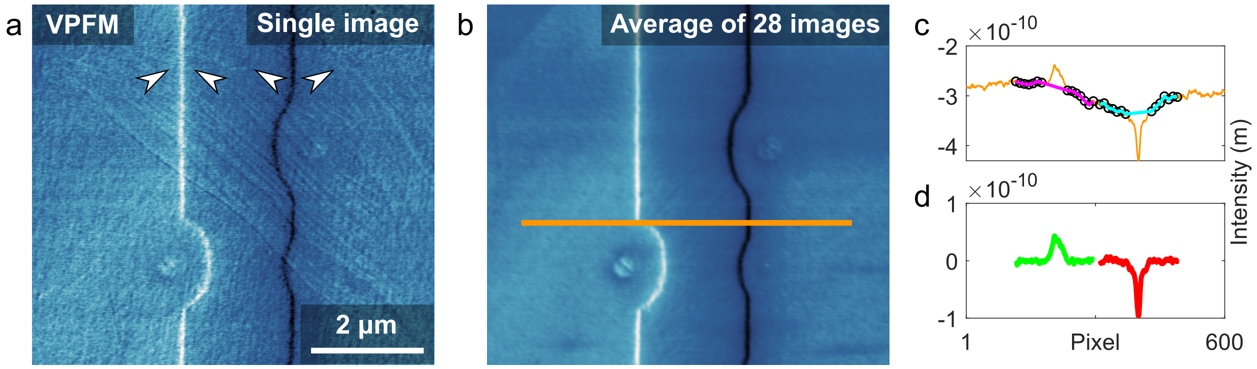


Figure S9: **Piezoresponse of the bended domain walls.** a) Single VPFM image. b) An average of 28 VPFM images. c) Cross-section from b) with baselines for the two peaks. d) Cross-section from c) with baselines subtracted.

# Supplementary References

[1] Perdew, J.P., Ruzsinszky, A., Csonka, G.I., Vydrov, O.A., Scuseria, G.E., Constantin, L.A., Zhou, X., Burke, K.: Restoring the density-gradient expansion for exchange in solids and surfaces. Physical review letters 100(13), 136406 (2008)

[2] Kresse, G., Furthmüller, J.: Efficient iterative schemes for ab initio total-energy calculations using a plane-wave basis set. Physical review B 54(16), 11169 (1996)

[3] Soergel, E.: Piezoresponse force microscopy (PFM). Journal of Physics D: Applied Physics 44(46), 464003 (2011)
